# Supplementary material for: FMGS: Foundation Model Embedded 3D Gaussian Splatting for Holistic 3D Scene Understanding
Source: arXiv:2401.01970 source file (2024-05-03)
Supplement: Supplementary file 1 [file 5_appendix.tex]

\begin{appendices}

\end{appendices}
